# Supplementary material for: Interactions par franchissement gr\^ace a un syst\`eme de suivi du regard
Source: arXiv:2504.13844 source file (2025-02-07)
Supplement: Supplementary file 1 [file 10_Appendix.tex]

\appendix \chapter{Appendix} 

Appendix goes here...
